# Supplementary material for: Absence of Luther-Emery Superconducting Phase in the Three-Band Model for Cuprate Ladders
Source: arXiv:2010.10609 ancillary file (2021-09-13)
Supplement: Supplementary file 1 [file supplemental.pdf]

# Absence of Luther-Emery Superconducting Phase in the Three-Band Model for Cuprate Ladders

Jeong-Pil Song,[1] S. Mazumdar,[1] and R. Torsten Clay[2]

[1] *Department of Physics, University of Arizona, Tucson, AZ 85721*

[2] *Department of Physics and Astronomy and HPC$^2$ Center for Computational Sciences, Mississippi State, MS 39762*

(Dated: August 31, 2021)

## S.1. CHARGES AND SPIN GAPS

For each parameter set we performed Density Matrix Renormalization Group (DMRG) calculations for increasing values of the bond dimension *m*. Our DMRG code used the ITensor library [S1] and conserved both particle number and $S_z$. For the longer ladders our calculations used the parallel algorithm described in [S2]. For smaller values of *m* ($m \lesssim 1600$) we performed a large number of sweeps (50–100) at each *m* value. We also added noise to the DMRG process for the first several sweeps to help ensure that the calculation did not become stuck in a local minima. The calculations for charge densities and spin gaps used a DMRG bond dimension of up to $m = 5600$; for the pair-pair correlations (see Section S.2) we used an *m* of up to 19000.

The average charge densities on Cu and O sites (presented in Table I in the main paper) converge very rapidly in truncation error and ladder length. In Fig. S1 we show a typical size extrapolation of the average charge densities as a function of the inverse ladder length $1/L$ (*L* is the number of ladder rungs).

To calculate the spin gaps $\Delta_S$ we first extrapolated the $S_z = 0$ and $S_z = 1$ energies with a linear extrapolation in DMRG truncation error and then performed a finite-size scaling versus $1/L$. In Fig. S2 we show a typical extrapolation in truncation error for an undoped ($\delta = 0$) 40-rung ladder for $U_d = 8$, $U_p = 3$, and $t_{pp} = 0.0$. We used a linear extrapolation in truncation error including only points with truncation error $\lesssim 1.0\times10^{-6}$.

Figs. S3-S5 show the finite-size scaling of the $\Delta_S$ data presented in Fig. 2 of the main paper. In all cases we used a quadratic fit in $1/L$ for the finite-size extrapolation. Here we used ladder lengths of up to 40, except for $\delta = 0.0625$, where we included ladders of length up to $L = 64$. For all parameters we found that a quadratic function in $1/L$ fit the data well.

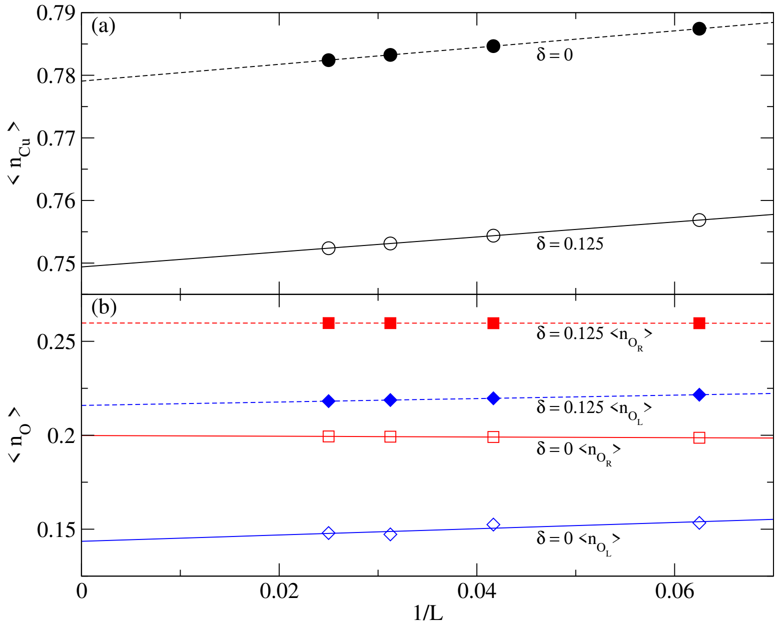


FIG. S1: Average charge density on Cu, $O_R$, and $O_L$ sites as a function of the inverse ladder length $1/L$, for $U_d = 8$, $U_p = 3$, $t_{pp} = 0.5$, $t_{dp} = 1$, and $t^{\perp}_{dp} = 1$. Open and filled symbols are for $\delta = 0$ and $\delta = 0.125$, respectively. Circles, squares, and diamonds correspond to densities of Cu, $O_R$, and $O_L$. The lines are linear fits.

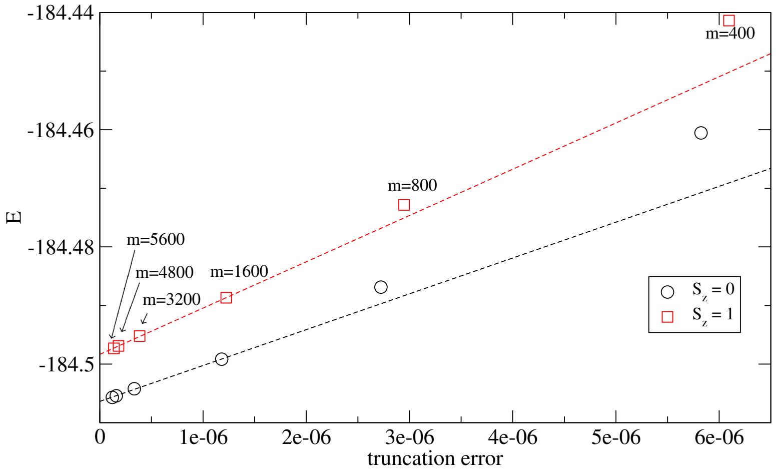


FIG. S2: Energy as a function of DMRG truncation error for $U_{\rm d}$ = 8, $U_{\rm p}$ = 3, $t_{\rm dp}^{\perp} = 1$, $t_{\rm pp}$ = 0.0, and $\delta = 0$ for a 40-rung ladder. Circles (squares) correspond to E($S_z$ = 0) and (E($S_z$ = 1)), respectively. The dashed lines are linear fits.

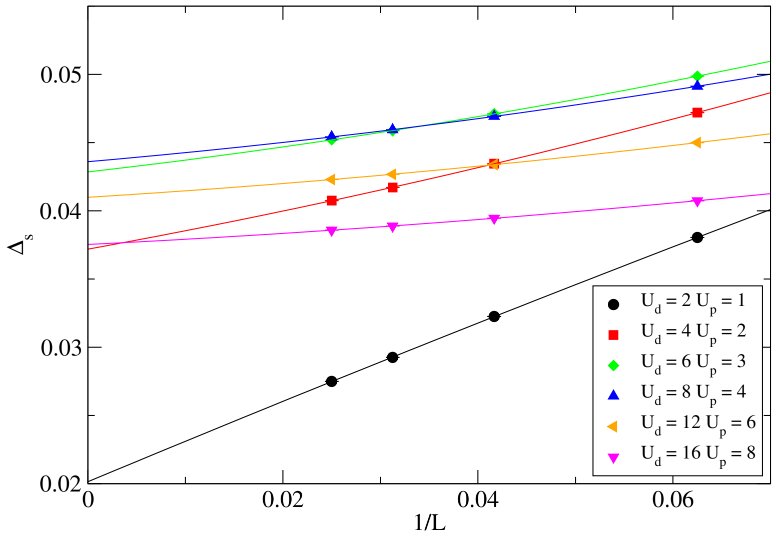


FIG. S3: Finite size extrapolation of the undoped ladder spin gap $\Delta_{\rm S}$ (see Fig. 2(a) in the main paper) for $U_{\rm p} = \frac{1}{2}U_{\rm d}$, $t_{\rm dp}^{\perp} = 1$, and $t_{\rm pp}$ = 0.5. The lines are quadratic fits.

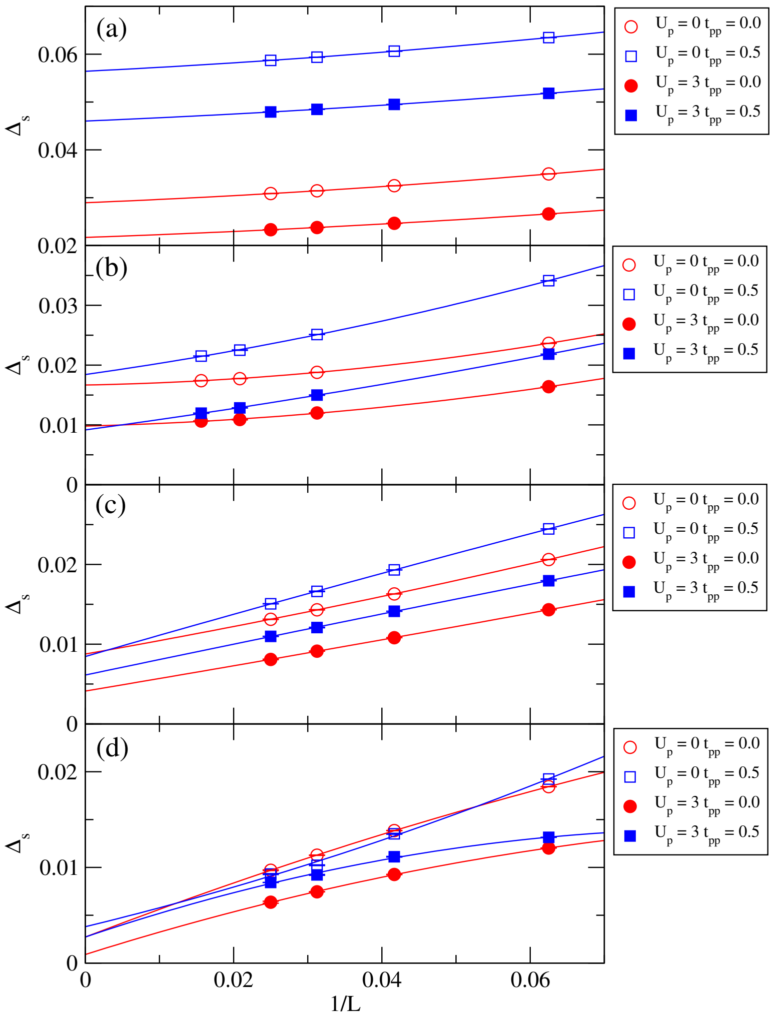


FIG. S4: Finite size extrapolation of the spin gap $\Delta_S$ (see Fig. 2(b) in the main paper) for $U_d = 8$ and $t_{dp}^{\perp} = 1$. In panel (a) $\delta = 0$, (b) $\delta = 0.0625$, (c) $\delta = 0.125$, and (d) $\delta = 0.25$. Open and filled symbols are for $U_p = 0$ and $U_p = 3$, respectively. Circles (squares) correspond to $t_{pp} = 0.0$ ($t_{pp} = 0.5$). The lines are quadratic fits.

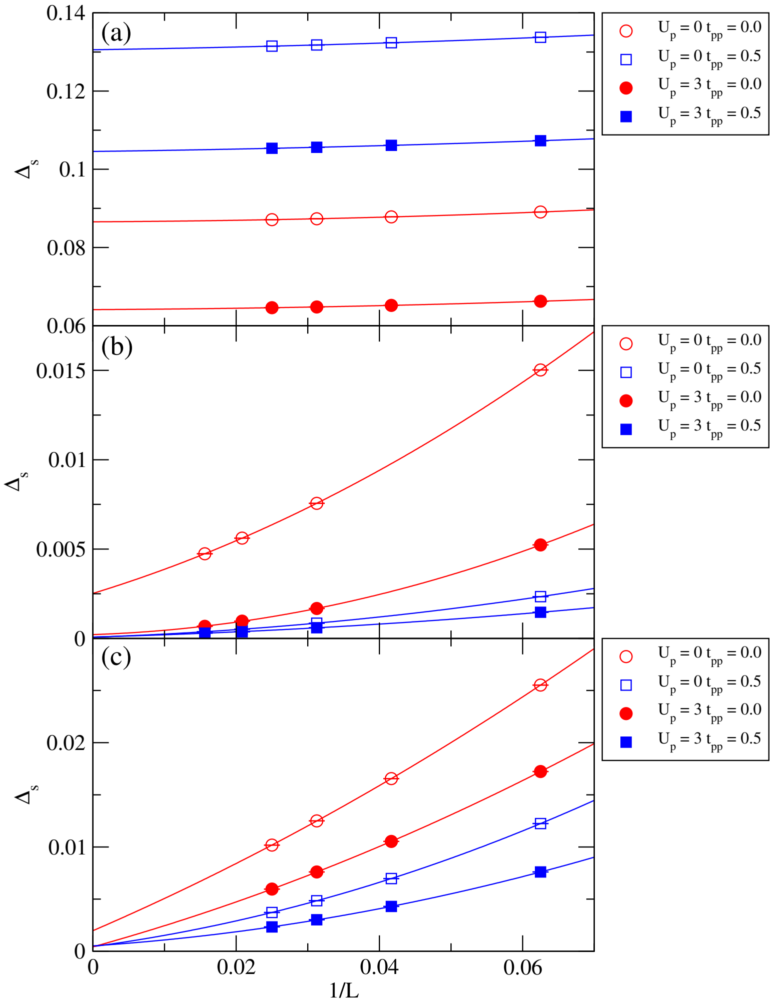


FIG. S5: Finite size extrapolation of the spin gap $\Delta_S$ (see Fig. 2(b) in the main paper) for $U_d = 8$ and $t_{dp}^{\perp} = 1.25$. In panel (a) $\delta = 0$, (b) $\delta = 0.0625$, and (c) $\delta = 0.125$. Open and filled symbols are for $U_p = 0$ and $U_p = 3$, respectively. Circles (squares) correspond to $t_{pp} = 0.0$ ($t_{pp} = 0.5$). The lines are quadratic fits.

## S.2. PAIR-PAIR CORRELATIONS

### S.2.1. Fitting of pair-pair correlations

This section explains the procedure we used to fit the power law exponent $\alpha$ reported in the main text. The data shown here are for one set of parameters: ladder length 96 rungs, $U_\mathrm{d} = 8$, $U_\mathrm{p} = 0$, $t_\mathrm{pp} = 0$, and doping $\delta = 0.125$. The extrapolations for other parameters are similar. For each value of $P_{i,j}$ where $i$ and $j$ are rung indices and $r = |i-j|$, we performed an extrapolation to zero DMRG truncation error. Typical extrapolations are shown in Fig. S6. The minimum truncation error reached for each parameter set was of order $1\times10^{-8}$ or smaller. For each $P_{i,j}$ we performed a linear extrapolation using the three smallest truncation error data points. The reported values of the power law exponent, $\alpha$, were determined with a least-squares fit using distances between $r = 10$ and $r = L/2 = 48$.

Because the DMRG calculations are performed using open boundary conditions, for each $r$ we performed an averaging over $N_\mathrm{avg}$ different $P_{i,j}$ with $r = |i-j|$ [S3]. The open boundaries lead to oscillations in $P(r)$ as a function of $r$, which increases the uncertainty in fitting the power law decay $P(r) \sim r^{-\alpha}$. These oscillations are reduced by the averaging process. For the results presented in the main paper, we took rungs $i$ and $j$ equally spaced about the center of the ladder with $N_\mathrm{avg}$=11 (12) for odd (even) $r$. In Fig. S7 we compare the truncation-error extrapolated and averaged $P(r)$ (reported in Fig. 4(a) of the main paper) with the averaged $P(r)$ without truncation error extrapolation. As $m$ increases $P(r)$ smoothly approaches the extrapolated $P(r)$. In Fig. S8 we used the extrapolated $P_{i,j}$ to calculate $P(r)$ with different values of $N_\mathrm{avg}$. Our choice of $N_\mathrm{avg}$ is the same as used in DMRG calculations on the one-band Hubbard ladder [S3]; as shown in Fig. S8, the choice of $N_\mathrm{avg}$ has little effect on the fitted value of of $\alpha$.

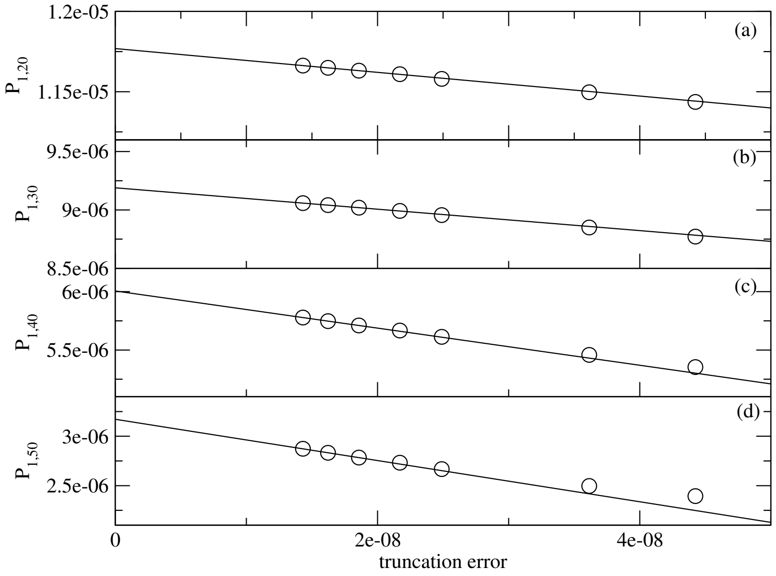


FIG. S6: Sample DMRG truncation error extrapolations of $P_{i,j}$ for a 96-rung ladder with $U_\mathrm{d}$ = 8, $U_\mathrm{p}$ = 0, $t_\mathrm{pp}$ = 0, and doping $\delta$ = 0.125. Panels (a)–(d) are for $\{i,j\}$= $\{1,20\}$, $\{1,30\}$, $\{1,40\}$, and $\{1,50\}$, respectively. In each case we used a linear extrapolation using the three smallest truncation error points.

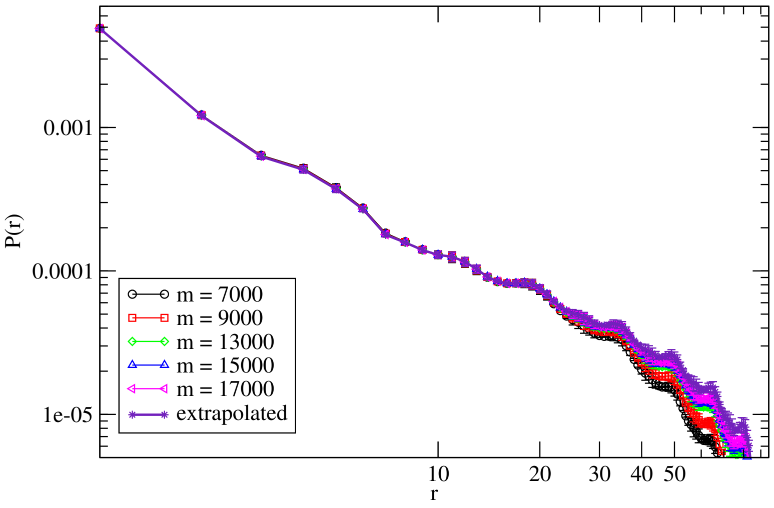


FIG. S7: Pair-pair correlation $P(r)$ versus $r$ for different DMRG bond dimension $m$. Here we used $N_{avg}$ = 11 or 12 (see text) for all points; truncation error extrapolation was only used for the "extrapolated" data set. Error bars here are calculated from the standard deviation of the averaged values of $P_{i,j}$. Other parameters are the same as in Fig. S6.

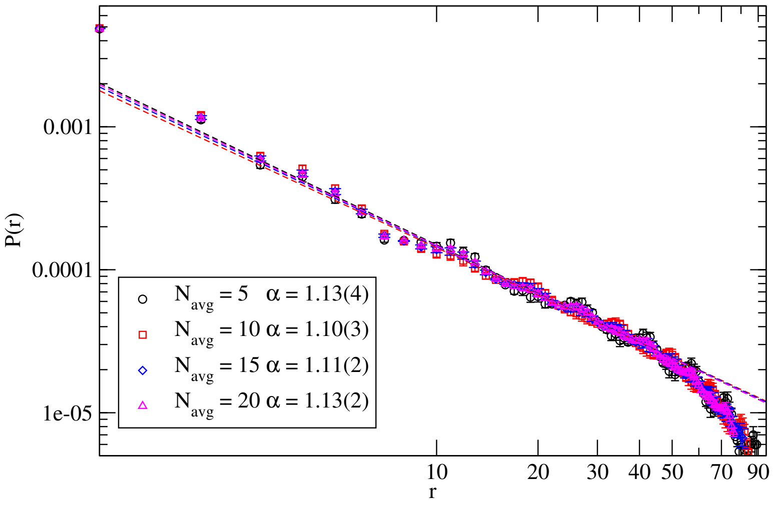


FIG. S8: Pair-pair correlation $P(r)$ versus $r$ for different $N_{avg}$. Parameters are the same as in Figs. S7 and S6. $P_{1,j}$ was first extrapolated to zero DMRG truncation error as described in the text. Error bars here are calculated from the standard deviation of the averaged values of $P_{i,j}$. The lines are linear fits over the range $10 \leq r \leq \frac{L}{2}$.

## S.3. DISTANCE DECAY OF DENSITY OSCILLATIONS

In Figs. S9-S13 we show fits to the amplitude of density oscillations $\delta n$ for each of the parameters in Table II of the paper.

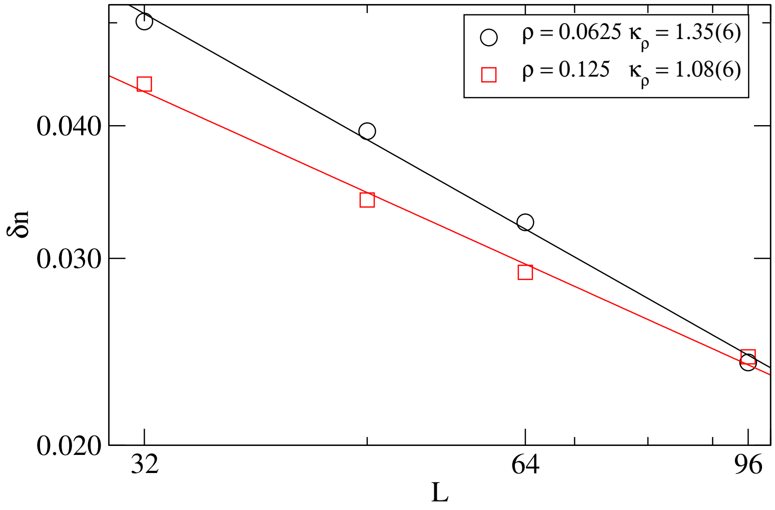


FIG. S9: Amplitude of density oscillations in the ladder center versus number of ladder rungs $L$ for $U_{\rm p} = 0$ and $t_{\rm pp} = 0$.

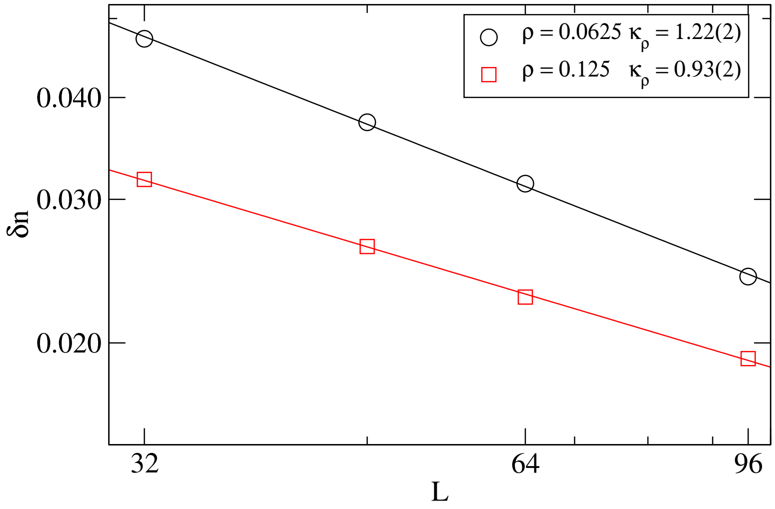


FIG. S10: Same as Fig. S9 for $U_{\rm p} = 0$ and $t_{\rm pp} = 0.5$.

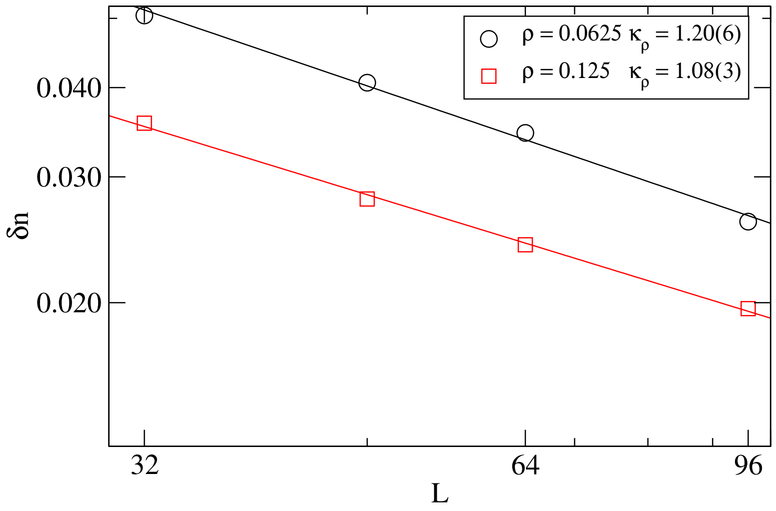


FIG. S11: Same as Fig. S9 for $U_\mathrm{p} = 3$ and $t_\mathrm{pp} = 0$.

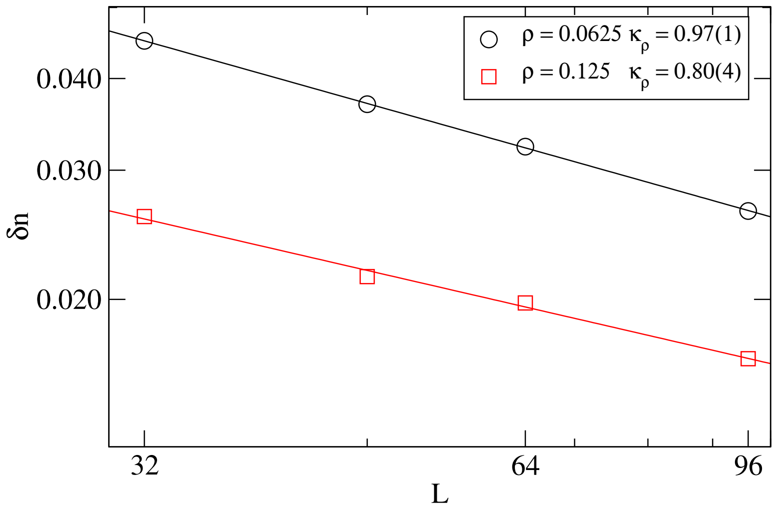


FIG. S12: Same as Fig. S9 for $U_\mathrm{p} = 3$ and $t_\mathrm{pp} = 0.5$.

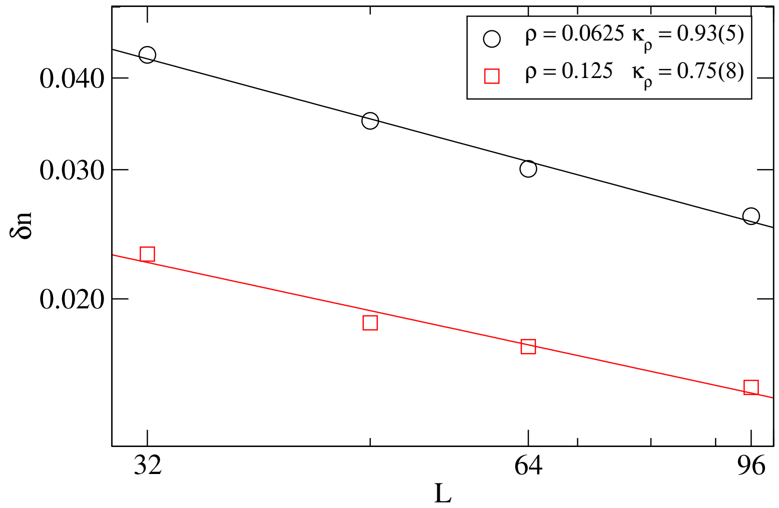


FIG. S13: Same as Fig. S9 for $U_{\rm p} = 4$ and $t_{\rm pp} = 0.6$.

[S1] Matthew Fishman, Steven R. White, and E. Miles Stoudenmire. The ITensor software library for tensor network calculations. preprint https://arxiv.org/abs/2007.14822, 2020.
[S2] E. M. Stoudenmire and S. R. White. Real-space parallel density matrix renormalization group. *Phys. Rev. B*, 87:155137, 2013.
[S3] M. Dolfi, B. Bauer, S. Keller, and M. Troyer. Pair correlations in doped Hubbard ladders. *Phys. Rev. B*, 92:195139, 2015.
